# Supplementary material for: Emergent hyperuniformity in periodically-driven emulsions
Source: arXiv:1504.04638 source file (2015-04-28)
Supplement: Supplementary file 1 [file SupMat.pdf]

# Emergent hyperuniformity in periodically-driven emulsions — Supplemental Documentation —

Joost H. Weijs[1], Raphaël Jeanneret[2], Rémi Dreyfus[3], and Denis Bartolo[1]
[1] *Laboratoire de Physique de l'École Normale Supérieure de Lyon, France*
[2] *Department of Physics, University of Warwick, Coventry CV4 7AL, United Kingdom*
[3] *Complex Assemblies of Soft Matter, CNRS-Solvay-UPenn UMI 3254, Bristol, Pennsylvania 19007-3624, USA*
(Dated: April 17, 2015)

This document contains additional information and data on the paper "Emergent hyperuniformity in periodically-driven emulsions" by Weijs, Jeanneret, Dreyfus, and Bartolo. In this document we provide the measured length-scale for translational order $\ell_{g(r)}$ for both the experiments and the numerical simulations and the structural relaxation time $\tau_{g(r)}$ for the numerical simulations. Furthermore, we provide a detailed explanation of the numerics, focusing on the treatment of the boundary conditions, and a brief explanation on the method used to measure the hyperuniformity extent $\ell_{\text{HU}}$ in the paper.

## COMPARISON OF LENGTH-SCALES $\ell_{g(r)}$ AND $\ell_{HU}$

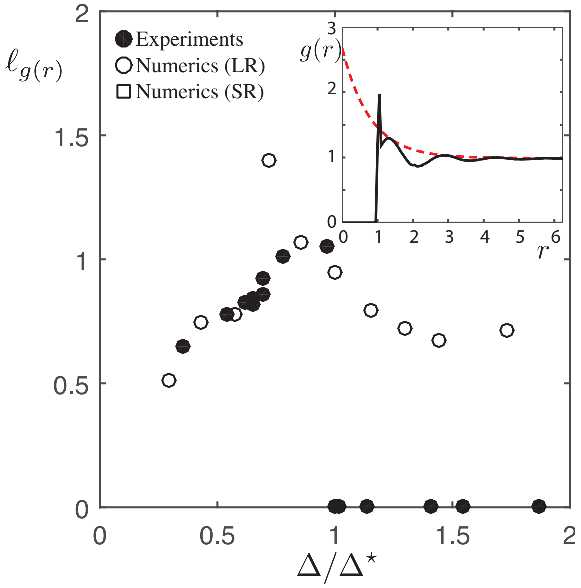


FIG. 1. Translational order $[g(r)]$ liquid structure length scale $\ell_{g(r)}$ at varying driving amplitude $\Delta$ for the experiments and the numerics with long-ranged interactions. For $\Delta > \Delta^\star$ the liquid structure breaks down. Lines are drawn as a guide the eye. The inset shows an example fit of the liquid peaks of $g(r)$, used to determine $\ell_{g(r)}$.

In Fig. 1 we show how the extent of the liquid-like structure $\ell_{g(r)}$ varies with the driving amplitude $\Delta$. This extent is measured by fitting an exponential

$$g_p(r) = a \exp\left(-\frac{r}{\ell_{g(r)}}\right) + 1 \tag{1}$$

to the liquid-peaks of the pair-correlation function $g(r)$. One of these fits is shown in the inset of Fig. 1. For $\Delta > \Delta^\star$ the liquid-like structure breaks down [1]. The experiments and the simulations show very similar trends, the length always remains below $\ell_{g(r)} = 2a$, much shorter than the hyperuniformity length-scales $\ell_{\text{HU}}$ reported in the main document. This is also the case for the short-ranged numerics, except around $\Delta = \Delta^\star$ where a sharp increase of $\ell_{g(r)}$ occurs. Nevertheless, for all driving amplitudes we find also for these simulations $\ell_{g(r)} \ll \ell_{\text{HU}}$.

## RELAXATION TIME FOR THE NUMERICS

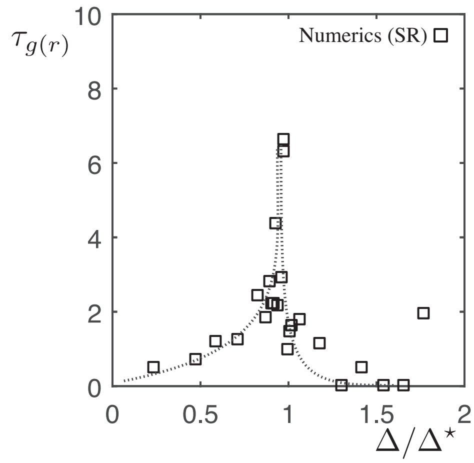


FIG. 2. Relaxation time $\tau_{g(r)}$ of the contact peak of the pair correlation function $g(r = a)$ for the short-range numerics. There is a clear peak at $\Delta = \Delta^\star$, hinting towards critical behaviour. The lines are a guide to the eye to more easily distinguish the peak.

In Fig. 2 we show the structural relaxation time of the emulsion for the short-range numerics. These times were measured by fitting the value of the contact peak of the pair correlation function $g(r = a)$ to an exponential decay. To obtain sufficient statistics to compute $g(r)$ we averaged this quantity over the full course of the cycle, thus ensuring that we retain sufficient time-resolution. The trend is that this structural relaxation time sharply increases at the transition yet it remains rather short. Much larger simulations would be needed to test quantitatively a potential critical-slowing-down effect. Simulations with long-range interactions do not show any significant variation of this relaxation time which remains very low at all driving amplitudes. In the experiments the relaxation time of all quantities is always shorter that the stabilization time of the imposed flow rate that is of the order of 20 cycles. This time is mostly set by the compliance of the microfluidic tubing.

## NUMERICAL DETAILS

The numerics consisted of a straightforward fixed-timestep Euler integration routine of the equation of motion:

$$\dot{\mathbf{r}}_\mathbf{i} = \mu \left( \mathbf{u_0}(t) + \sum_{j\neq i} \frac{2\hat{\mathbf{r}}_\mathbf{ij}\hat{\mathbf{r}}_\mathbf{ij} - \mathbb{1}}{2\pi|\mathbf{r}_\mathbf{ij}|^2} \cdot \boldsymbol{\sigma}_j \right) \ . \tag{2}$$

Fully solving the above equation of motion involves a computationally expensive matrix inversion, as $\boldsymbol{\sigma}_j$ itself depends on the location of all other particles including particle $i$:

$$\boldsymbol{\sigma}_j = \sigma(\dot{\mathbf{r}}_j - \mathbf{u}(\mathbf{r}_j)) \ , \tag{3}$$

with

$$\mathbf{u}_0 \equiv u_0(t)\hat{\mathbf{x}} \tag{4}$$

where $u_0(t)$ is the sinusoidal driving done by the syringe pump in the experiment. The values of $\dot{\mathbf{r}}_j$ and $\mathbf{u}(\mathbf{r})$ have contributions from both the driving flow and all induced dipoles. However the induced flows by other dipoles a higher order term than the driving flow, it turns out –by comparing simulation results– that we can neglect this higher order term (so: $\dot{\mathbf{r}}_j \approx \mu\mathbf{u}_0$ and $\mathbf{u}(\mathbf{r}) \approx \mathbf{u}_0$) and therefore:

$$\boldsymbol{\sigma}_j \approx \sigma\mathbf{u}_0(\mu - 1) \ , \tag{5}$$

For the simulations in this work, the following boundary conditions were applied: no-flux boundary conditions at $y = \pm W/2$ and periodic boundary conditions in the $x$-direction, see Fig. 3. The no-flux boundary conditions induce

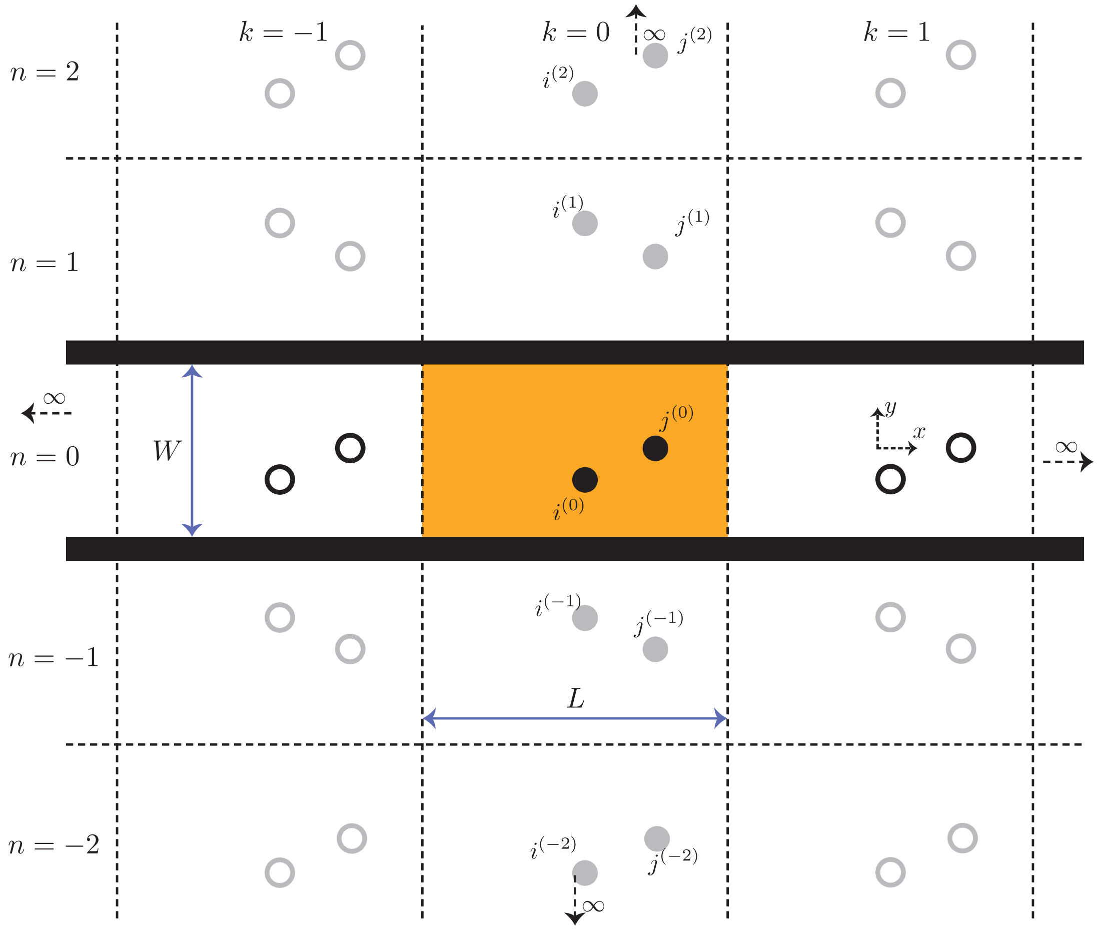


FIG. 3. Representation of the simulations. The orange box in the center contains the physical simulation domain, with periodic boundary condition in the driving flow ($x$)-direction and solid walls in the transverse flow ($y$)-direction. Two sample particles are drawn. The walls cause of virtual images of the real particles, to account for the no-flux boundary condition at the solid walls. Because these virtual images also form additional images due to the presence of the second wall, an infinite "column" of images is formed as shown in the image. The periodic boundary conditions then repeat this column by translation in the $x$ and $-x$ directions. Since the interactions are long-ranged, all real and virtual particles must be accounted for in the simulations.

an infinite series of image dipoles in the $+y$ and $-y$ directions for all particles. This leads to an infinitely long 'column' of dipoles which is repeated in the $-x$ and $+x$-directions. This is displayed in Fig. 3, where the 'live' cell (containing the real dipoles) is shaded orange. Because the number of virtual dipoles is infinite, we use a method similar as described in [2] to compute the full interactions at feasible computational cost. This method consists of separating the interactions that occur at smaller and larger distances. The interactions that occur at short distances (and which are therefore relatively strong) are calculated explicitly, and therefore exact. The contribution due to the (virtual) dipoles at greater distances are pre-computed. This takes the form of a tensor-field, of which the values are calculated at discrete points and during the simulation interpolation is used to calculate the approximate value of the tensor-field based on the position of the particle-pair $ij$ that is being considered [Eq. (2)]. The image-dipoles due to the no-flux boundary conditions are located at:

$$x_i^{(n)} = x_i^{(0)}$$
$$y_i^{(n)} = \begin{cases} nW - y_i^{(0)} & \text{if } n \text{ odd} \\ nW + y_i^{(0)} & \text{if } n \text{ even} \end{cases} \tag{6}$$

Therefore, in order to avoid having to calculate a field that depends on three variables, we are required to calculate *two* tensor-fields to account for the far-field interactions: one that accounts for the even dipoles, and one for the odd dipoles. The first step is to calculate the interactions due to a single column of even or odd images, at a position

$\mathbf{r}$ induced by a real dipole at $\mathbf{r}_i$ and its images at $\mathbf{r_i^{(n)}}$, whose positions are dictated by Eq. (6). For each dipole $n$: $\Delta x \equiv (\mathbf{r}-\mathbf{r_i^{(n)}})\cdot\hat{\mathbf{x}} = x - x_i$. Furthermore, for even $n$: $\Delta y_n \equiv (\mathbf{r}-\mathbf{r_i^{(n)}})\cdot\hat{\mathbf{y}} = y - y_i^{(n)} = y - nW - y_i^{(0)} = \Delta y - nW$, and so for odd $n$: $\Delta y_n = y - nW + y_i^{(0)} = \Delta y' - nW$.

For even $n$ we get:

$$G^{\text{column}}_{\text{even}}(\Delta x,\Delta y) = \frac{1}{2\pi}\sum_{\substack{n=-\infty,\\ n\ \text{even}}}^{\infty}\begin{pmatrix} \frac{2\Delta x\Delta x}{(\Delta x^2+\Delta y_n^2)^{3/2}} - \frac{1}{(\Delta x^2+\Delta y_n^2)} & \frac{2\Delta x\Delta y_n}{(\Delta x^2+\Delta y_n^2)^{3/2}} \\ \frac{2\Delta y_n\Delta x}{(\Delta x^2+\Delta y_n^2)^{3/2}} & \frac{2\Delta y_n\Delta y_n}{(\Delta x^2+\Delta y_n^2)^{3/2}} - \frac{1}{(\Delta x^2+\Delta y_n^2)}\end{pmatrix}$$

$$= \frac{1}{2\pi}\sum_{\substack{n=-\infty\\ n\ \text{even}}}^{\infty}\begin{pmatrix} \frac{2\Delta x\Delta x}{(\Delta x^2+(\Delta y-nW)^2)^{3/2}} - \frac{1}{(\Delta x^2+(\Delta y-nW)^2)} & \frac{2\Delta x(\Delta y-nW)}{(\Delta x^2+(\Delta y-nW)^2)^{3/2}} \\ \frac{2(\Delta y-nW)\Delta x}{(\Delta x^2+(\Delta y-nW)^2)^{3/2}} & \frac{2(\Delta y-nW)^2}{(\Delta x^2+(\Delta y-nW)^2)^{3/2}} - \frac{1}{(\Delta x^2+(\Delta y-nW)^2)}\end{pmatrix}$$

$$= \frac{\pi}{16W^2}\begin{pmatrix} \operatorname{csch}\left(\frac{\pi(\Delta x-i\Delta y)}{2W}\right)^2 + \operatorname{csch}\left(\frac{\pi(\Delta x+i\Delta y)}{2W}\right)^2 & -i\left(\operatorname{csch}\left(\frac{\pi(\Delta x-i\Delta y)}{2W}\right)^2 - \operatorname{csch}\left(\frac{\pi(\Delta x+i\Delta y)}{2W}\right)^2\right) \\ -i\left(\operatorname{csch}\left(\frac{\pi(\Delta x-i\Delta y)}{2W}\right)^2 - \operatorname{csch}\left(\frac{\pi(\Delta x+i\Delta y)}{2W}\right)^2\right) & f_{\text{even}}(\Delta x,\Delta y,W)\end{pmatrix} \tag{7}$$

And for $n$ is odd:

$$G^{\text{column}}_{\text{odd}}(\Delta x,\Delta y') = \frac{1}{2\pi}\sum_{\substack{n=-\infty\\ n\ \text{odd}}}^{\infty}\begin{pmatrix} \frac{2\Delta x\Delta x}{(\Delta x^2+\Delta y_n^2)^{3/2}} - \frac{1}{(\Delta x^2+\Delta y_n^2)} & \frac{2\Delta x\Delta y_n}{(\Delta x^2+\Delta y_n^2)^{3/2}} \\ \frac{2\Delta y_n\Delta x}{(\Delta x^2+\Delta y_n^2)^{3/2}} & \frac{2\Delta y_n\Delta y_n}{(\Delta x^2+\Delta y_n^2)^{3/2}} - \frac{1}{(\Delta x^2+\Delta y_n^2)}\end{pmatrix}$$

$$= \frac{1}{2\pi}\sum_{\substack{n=-\infty\\ n\ \text{odd}}}^{\infty}\begin{pmatrix} \frac{2\Delta x\Delta x}{(\Delta x^2+(\Delta y'-nW)^2)^{3/2}} - \frac{1}{(\Delta x^2+(\Delta y'-nW)^2)} & \frac{2\Delta x(\Delta y'-nW)}{(\Delta x^2+(\Delta y'-nW)^2)^{3/2}} \\ \frac{2(\Delta y'-nW)\Delta x}{(\Delta x^2+(\Delta y'-nW)^2)^{3/2}} & \frac{2(\Delta y'-nW)^2}{(\Delta x^2+(\Delta y'-nW)^2)^{3/2}} - \frac{1}{(\Delta x^2+(\Delta y'-nW)^2)}\end{pmatrix}$$

$$= \frac{\pi}{16W^2}\begin{pmatrix} -\operatorname{sech}\left(\frac{\pi(\Delta x-i\Delta y')}{2W}\right)^2 + \operatorname{sech}\left(\frac{\pi(\Delta x+i\Delta y')}{2W}\right)^2 & i\left(\operatorname{csch}\left(\frac{\pi(\Delta x-i\Delta y')}{2W}\right)^2 - \operatorname{sech}\left(\frac{\pi(\Delta x+i\Delta y')}{2W}\right)^2\right) \\ i\left(\operatorname{csch}\left(\frac{\pi(\Delta x-i\Delta y')}{2W}\right)^2 - \operatorname{sech}\left(\frac{\pi(\Delta x+i\Delta y')}{2W}\right)^2\right) & f_{\text{odd}}(\Delta x,\Delta y',W)\end{pmatrix} \tag{8}$$

We did not print the $yy$-solutions $f$ even though they exist, because it is irrelevant [$\boldsymbol{\sigma}\cdot\hat{\mathbf{y}} = 0$, see Eqs. (4), (5)] and a very long expression.

The next step is to sum the *columns* to represent the periodic boundary conditions in the $x-$direction. This can be achieved by simply translating the coordinates with the simulation domain length $L$:

$$\Delta x_k = \Delta x + kL\ . \tag{9}$$

The complete tensor-fields are therefore:

$$G_{\text{even}} = \sum_{\substack{k=-\infty\\ k\ \text{even}}}^{\infty} G^{\text{column}}_{\text{even}}(\Delta x_k,\Delta y) \tag{10}$$

$$G_{\text{odd}} = \sum_{\substack{k=-\infty\\ k\ \text{odd}}}^{\infty} G^{\text{column}}_{\text{odd}}(\Delta x_k,\Delta y')\ . \tag{11}$$

Unfortunately no analytic solution exists for these expressions, so we compute the sum up to sufficiently high (and negative) $k = k_{max}$. From the expressions for $G^{\text{column}}_{\text{even}}$ and $G^{\text{column}}_{\text{odd}}$ [Eqs. (7), (8)] it is however clear there exists an exponential screening in the $x-$direction of characteristic length $2W$. Since $L > W$ we can therefore suffice with a limited number of columns. In this work we used an extremely high value of $k_{max} = 200$, which is by far sufficient to incorporate the periodic boundary conditions.

The very last step is to substract the *real* dipole contribution ($n = 0, k = 0$) from the computer tensor-fields, as these interactions will be computed explicitly during the simulation runs.

## MEASUREMENT OF $\ell_{\text{HU}}$

To measure the extent of the power laws in Fig. 3a-c of the paper, and thus the extent of the hyperuniform region $\ell_{rmHU}$, we use a method that separates the length associated with the curvature around the minimum of these curves form $\ell_{\text{HU}}$. The main idea is graphically depicted in Fig. 4 and consists of finding the intersection between the tangent curve at low $\ell$ with the minimum of $\Delta N_\ell^2$.

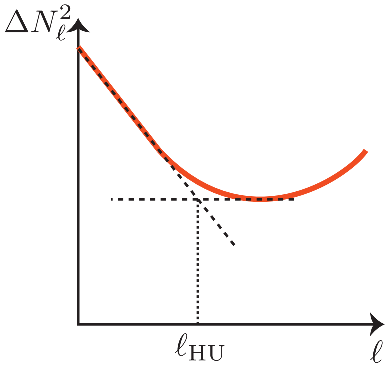


FIG. 4. Sketch to explain the procedure to determine $\ell_{\mathrm{HU}}$.

[1] R. Jeanneret and D. Bartolo, *Geometrically protected reversibility in hydrodynamic Loschmidt-echo experiments*, Nat. Comm. **5**, (2014).

[2] A. Lefauve and D. Saintillan, *Globally aligned states and hydrodynamic traffic jams in confined suspensions of active asymmetric particles*, Phys. Rev. E **89**, 021002 (2014).
